# Supplementary material for: Co-segmentation for Space-Time Co-located Collections
Source: arXiv:1701.08931 source file (2017-01-31)
Supplement: Supplementary file 2 [file appendix_supp.tex]

%!TEX root = supp_cvpr.tex
\section{Extending convex belief propagation}
%we first briefly review basic concepts of approximate inference and convex belief propagation. 

The variational interpretation for approximating Gibbs marginal probabilities follows the optimization program
%\johannes{There are probably 5 people in the world who will be able to understand this... Do we really need to provide this equation? I worry we might alienate our reviewers.}
\!{
\begin{eqnarray}
\footnotesize
\label{eq:cbp}
&& \arg \max_{b_i,b_{i,j}} \;\; \sum_{i,j, y_i,y_j} b_{i,j}(y_i,y_j) \theta_{i,j}(y_i,y_j) + \sum_{i,y_i} b_i(y_i) \theta_i(y_i) + \sum_{i \in V} c_i H(b_i) +  \sum_{i,j \in E} c_{i,j} H(b_{i,j}) \whitetxt{aaa}\\
&&  \mbox{s.t.} \;\;\; b_i(y_i), b_{i,j}(y_i,y_j) \ge 0, \;\; \sum_{y_i,y_j}b_{i,j}(y_i,y_j)=1, \sum_{y_i} b_i(y_i)=1,\sum_{y_j} b_{i,j}(y_i,y_j) = b_i(y_i). \nonumber
\end{eqnarray}
}
%\johannes{The equation is too wide, it overlaps the equation number. Break it differently or make the font smaller or remove white space using \textbackslash{}!}
%\johannes{what are the $b_i$?}
We denote by $N(i)$ the set of edges that connect to node $i$ and set $H(b_i) = -\sum_{y_i} b_i(y_i) \log b_i(y_i)$. Whenever the edges $E$ compose a graph without cycles and $c_{i,j}=1, c_i = 1-|N(i)|$ are the Bethe coefficients, the above variational program results in exact inference: the optimal beliefs $b_i(y_i)$ are the Gibbs marginal probabilities. For graphs with cycles this program approximates the inference, as its optimal beliefs approximate the Gibbs marginal probabilities. Importantly, when one uses positive entropy coefficients $c_i, c_{i,j} > 0$ the program is everywhere concave and have a unique global optimum. This global optimum can be attained efficiently, e.g., by message-passing algorithms \cite{Wainwright05-upper,Heskes06}. In our work we consider an extension of this program, to count for interactions across images: 

\begin{claim}
 Consider a program that augments Equation (\ref{eq:cbp}) with the non-linearities across images $\sum_{i,j \in E_b} \sum_{y_i} b_i(y_i) b_j(y_j)$.  
%\johannes{I want to be able to knock out equations like this one...}
\begin{eqnarray}
\label{eq:cbp2}
&& \arg \max_{b_i,b_{i,j}} \;\; \sum_{(i,j) \in E, y_i,y_j} b_{i,j}(y_i,y_j) \theta_{i,j}(y_i,y_j) + \sum_{i \in V,y_i} b_i(y_i) \theta_i(y_i) + \\
&& \hspace{2cm} \sum_{i,j \in E_b} \sum_{y_i} b_i(y_i) b_j(y_j) + \sum_{i \in V} c_i H(b_i) +  \sum_{i,j \in E} c_{i,j} H(b_{i,j})  \nonumber \\ 
&&  \mbox{s.t.} \;\;\; b_i(y_i), b_{i,j}(y_i,y_j) \ge 0, \;\; \sum_{y_i,y_j}b_{i,j}(y_i,y_j)=1, \sum_{y_i} b_i(y_i)=1,\sum_{y_j} b_{i,j}(y_i,y_j) = b_i(y_i). \nonumber
\end{eqnarray}
Then this program is strictly concave if $c_{i,j} > 0$ and for any $i$ there holds $c_i > \lambda_{max}(E_b)$ where $E_b$ is the adjacency matrix between images and $\lambda_{max}(N_b)$ is its maximal eigenvalue. Moreover, a message-passing algorithm (performing block coordinate ascent over the beliefs of this program) is guaranteed to converge to the program's optimum. 
\end{claim}
\emph{Proof:} The concavity of the program is determined by the eigenvalues of its Hessian. A function is strictly concave if the eigenvalues of  its Hessian are negative. The Hessian of the linear terms vanishes and we do not consider it. The Hessian of the entropy function is a diagonal matrix whose entries are the minus of the inverse beliefs. Therefore the eigenvalues of the entropy's Hessian are at most $-1$. The Hessian of the mixing terms  $\sum_{i,j \in E_b} \sum_{y_i} b_i(y_i) b_j(y_j)$ is dominated by the Hessian of $E_b$. This is a convex-concave function whose convex element is determined by $ \lambda_{max}(E_b)$. To overcome this convexity it is sufficient to set $c_i > \lambda_{max}(E_b)$ for every $i$. The convergence to the global optimum follows the strict concavity and Proposition 2.7.1 in \cite{Bertsekas99}.   

The maximal eigenvalue of an adjacency matrix is at most its maximal degree, hence $\lambda_{max}(E_b) \le \max_j |N_b(j)|$. This gives a simpler condition to guarantee convergence which does not require the maximal eigenvalue of $E_b$, namely for any $i$ with $c_i > \max_j |N_b(j)|$.
